# Supplementary material for: A Computational Framework for Behavioral Assessment of LLM Therapists
Source: arXiv:2401.00820 source file (2024-11-28)
Supplement: Supplementary file 1 [file appendix-fig-5-client-vs-therapist.tex]

\begin{figure*}[t]
\includegraphics[width=\textwidth]{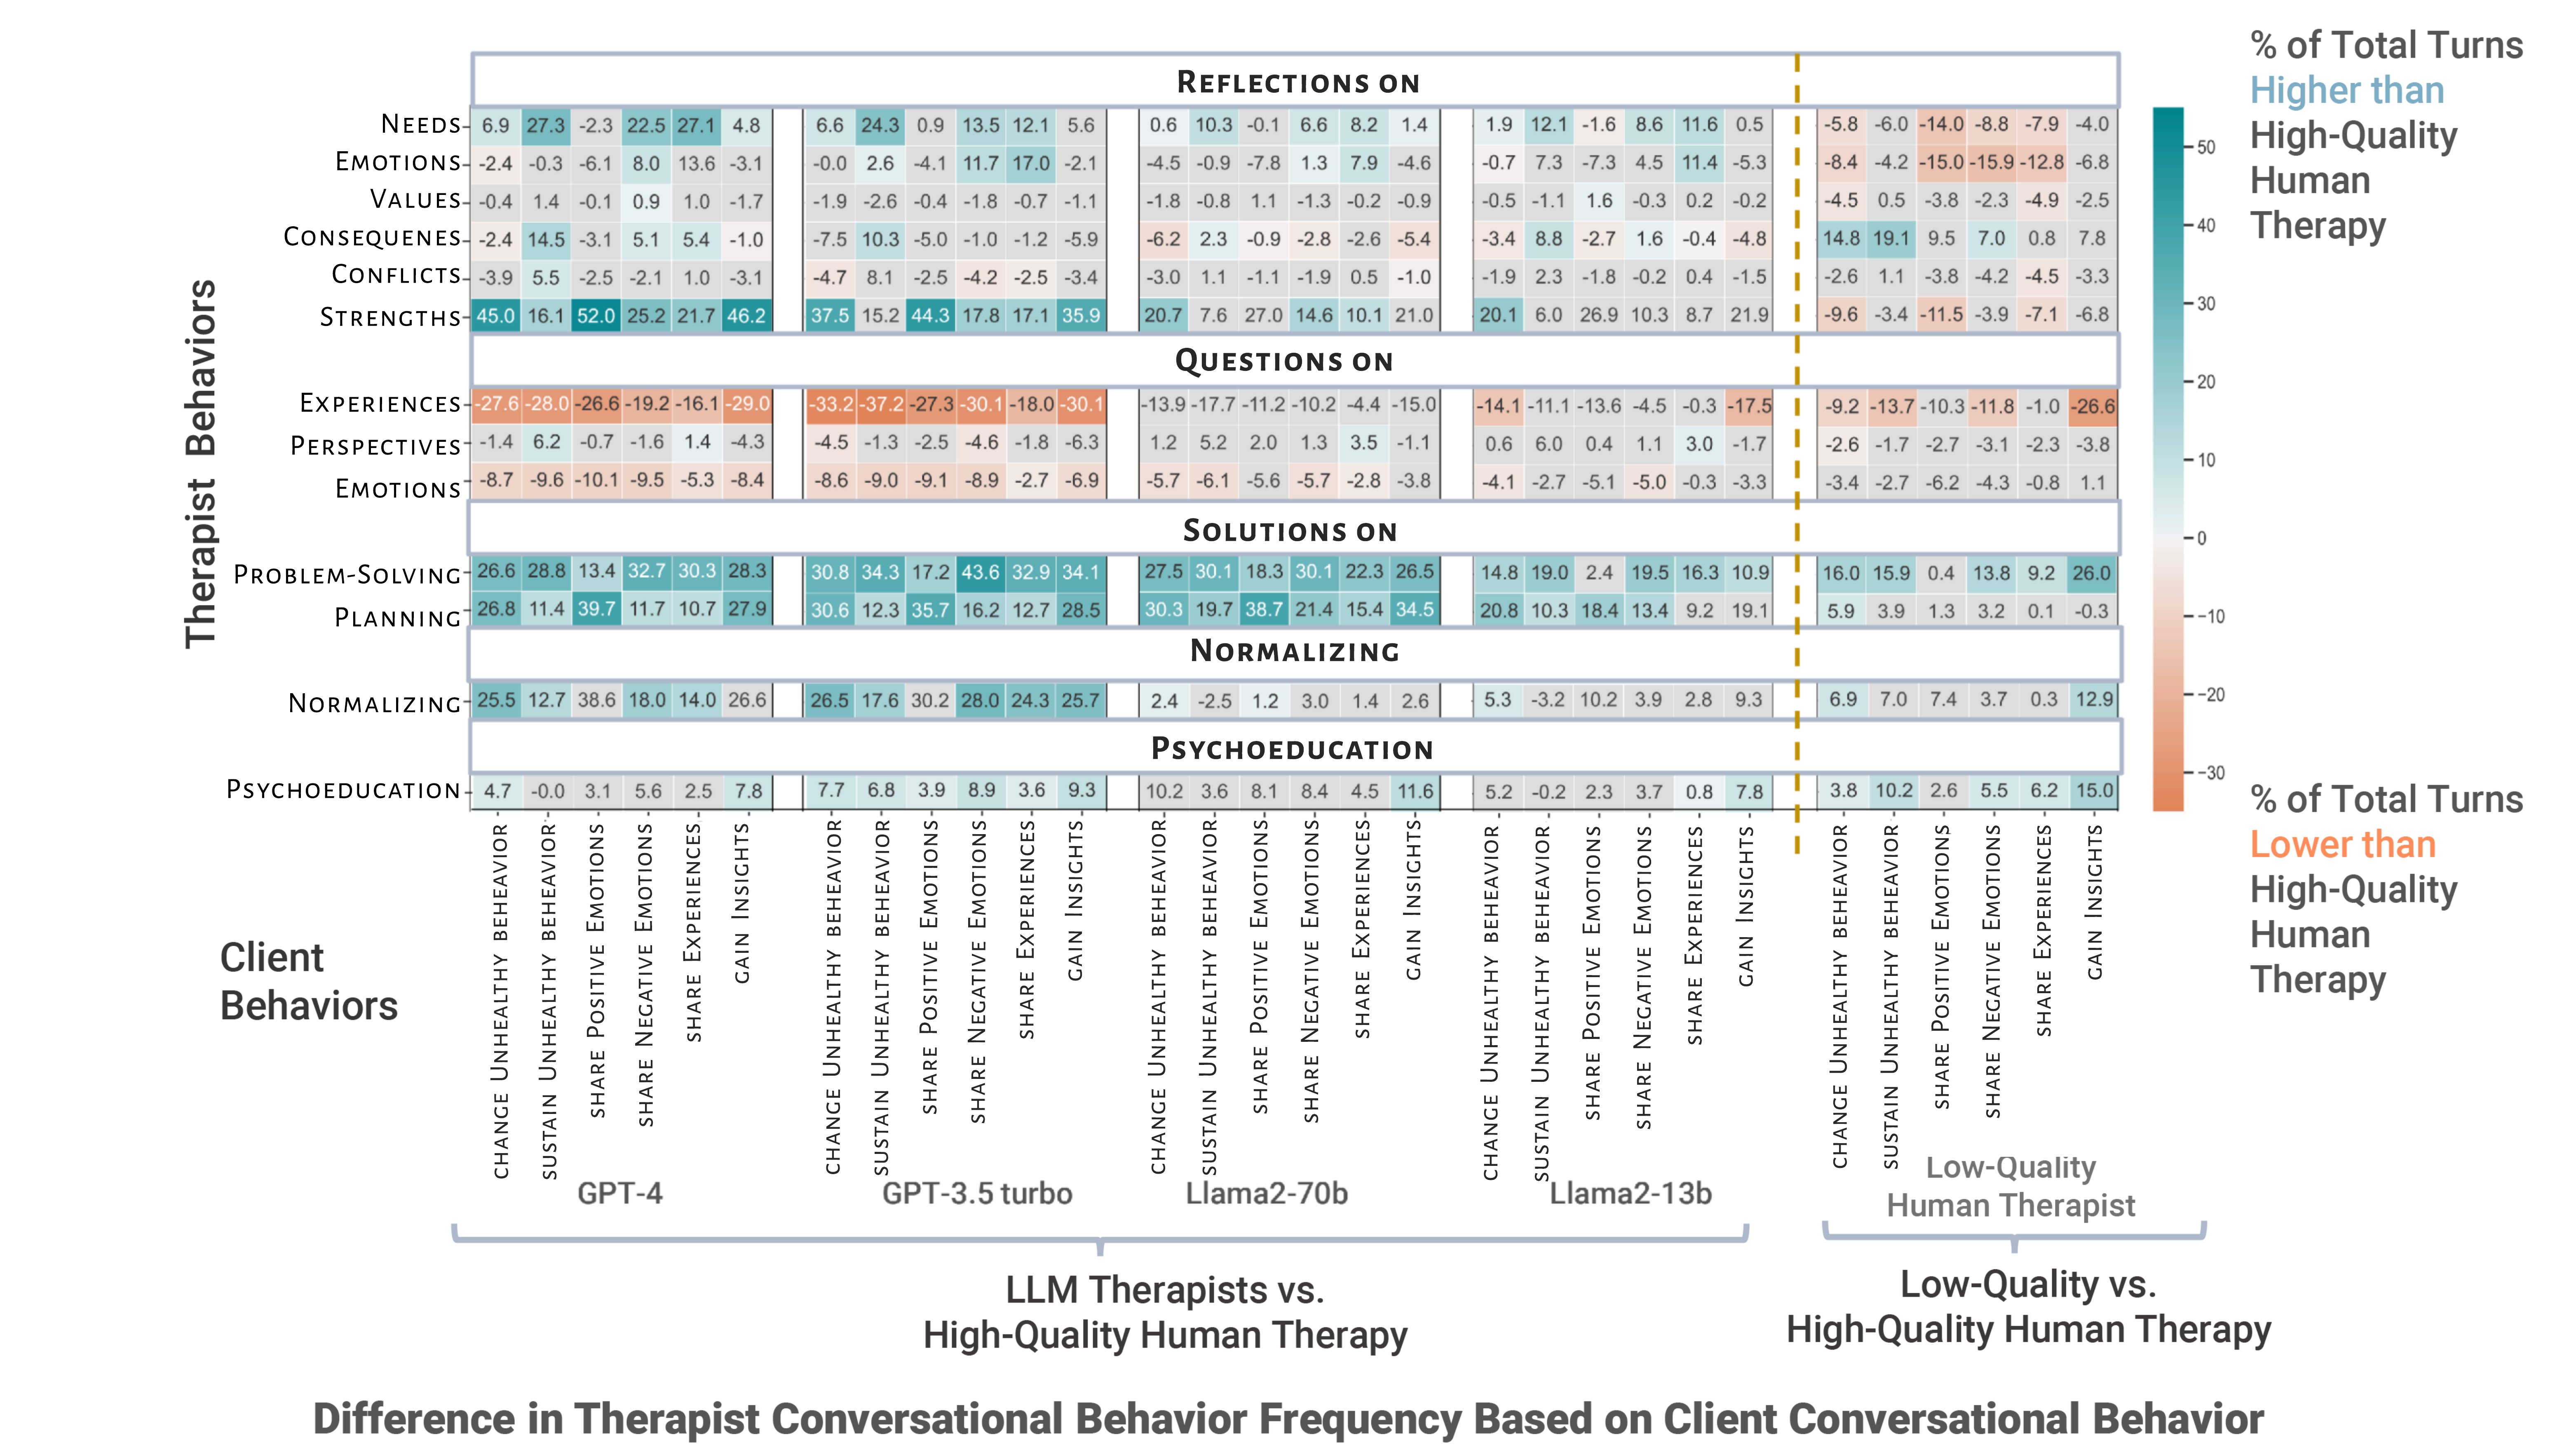}
\centering
\vspace{-15pt}
\caption{Difference between the frequency of conversational behaviors observed in LLM therapists (GPT-4, GPT-3.5-turbo, Llama2-70b, Llama2-13b) or low-quality human therapy \textit{in response to specific client behaviors} (\textit{Adaptability}), relative to the frequency of behavior observed in high-quality human therapy in the same case.
% the frequency of the behavior observed in high-quality human therapy in response to different client behaviors. 
Values $>0\%$ (colored in \textcolor{blueplot}{blue}) indicate significantly higher frequency whereas values $<0\%$ (colored in \textcolor{orangeplot}{orange}) indicate significantly lower frequency as compared to high-quality human therapy.
Values in \textcolor{gray}{gray} are not statistically significantly different from zero at p = 0.05 using Two-sided Student’s t-test. For instance, GPT-4 exhibits $7.8\%$ more \textsc{Psychoeducation} than high-quality human therapy when the client expresses \textsc{Gained Insights}. Here, one finding is that all LLMs respond with relatively higher \textsc{Psychoeducation} when compared with high-quality human therapy if the client expresses \textsc{Sustaining Unhealthy Behavior}, similar to low-quality human therapy. }
\label{appendix:fig:client-vs-therapist_avg}
\end{figure*}
% \tim{is this a rasterized graphic? Try to avoid}
% \tim{not clear whether these are absolute or relative and to what. the color bar annoation suggests relative to high quality human. make this more clear in caption}
% Values $>0\%$ (highlighted in \textcolor{blueplot}{blue}) indicate significantly higher observed occurrence of a particular behavior ($p < 0.05$) whereas values $<0\%$ (highlighted in \textcolor{orangeplot}{red}) indicate significantly lower observed occurrence of a particular behavior as compared to high-quality human therapists ($p < 0.05$).
% We find that if clients express sustaining unhealthy behavior, all LLMs respond with significantly higher reflections on consequences as compared to high-quality human therapists, a behavior also observed in low-quality human therapists. Moreover, if clients share positive emotions, all LLMs respond with significantly higher problem-solving, which is also observed in low-quality human therapists. Also, if clients share negative emotions or if they share life events, all LLMs respond with significantly higher reflections on emotions, which is in contrast to low-quality human therapists.

% \textbf{To interpret,} values \textcolor{blueplot}{\textbf{$>0\%$}} [\textcolor{orangeplot}{\textbf{$<0\%$}}] (highlighted in \textcolor{blueplot}{blue}[\textcolor{orangeplot}{orange}]) indicate significantly \textcolor{blueplot}{\textbf{higher}}[\textcolor{orangeplot}{\textbf{lower}}] observed occurrence of a particular behavior ($p < 0.05$). 
