# Supplementary material for: A Computational Framework for Behavioral Assessment of LLM Therapists
Source: arXiv:2401.00820 source file (2024-11-28)
Supplement: Supplementary file 2 [file appendix-fig-3-first-occ.tex]

\begin{figure*}[t]
\includegraphics[width=\textwidth]{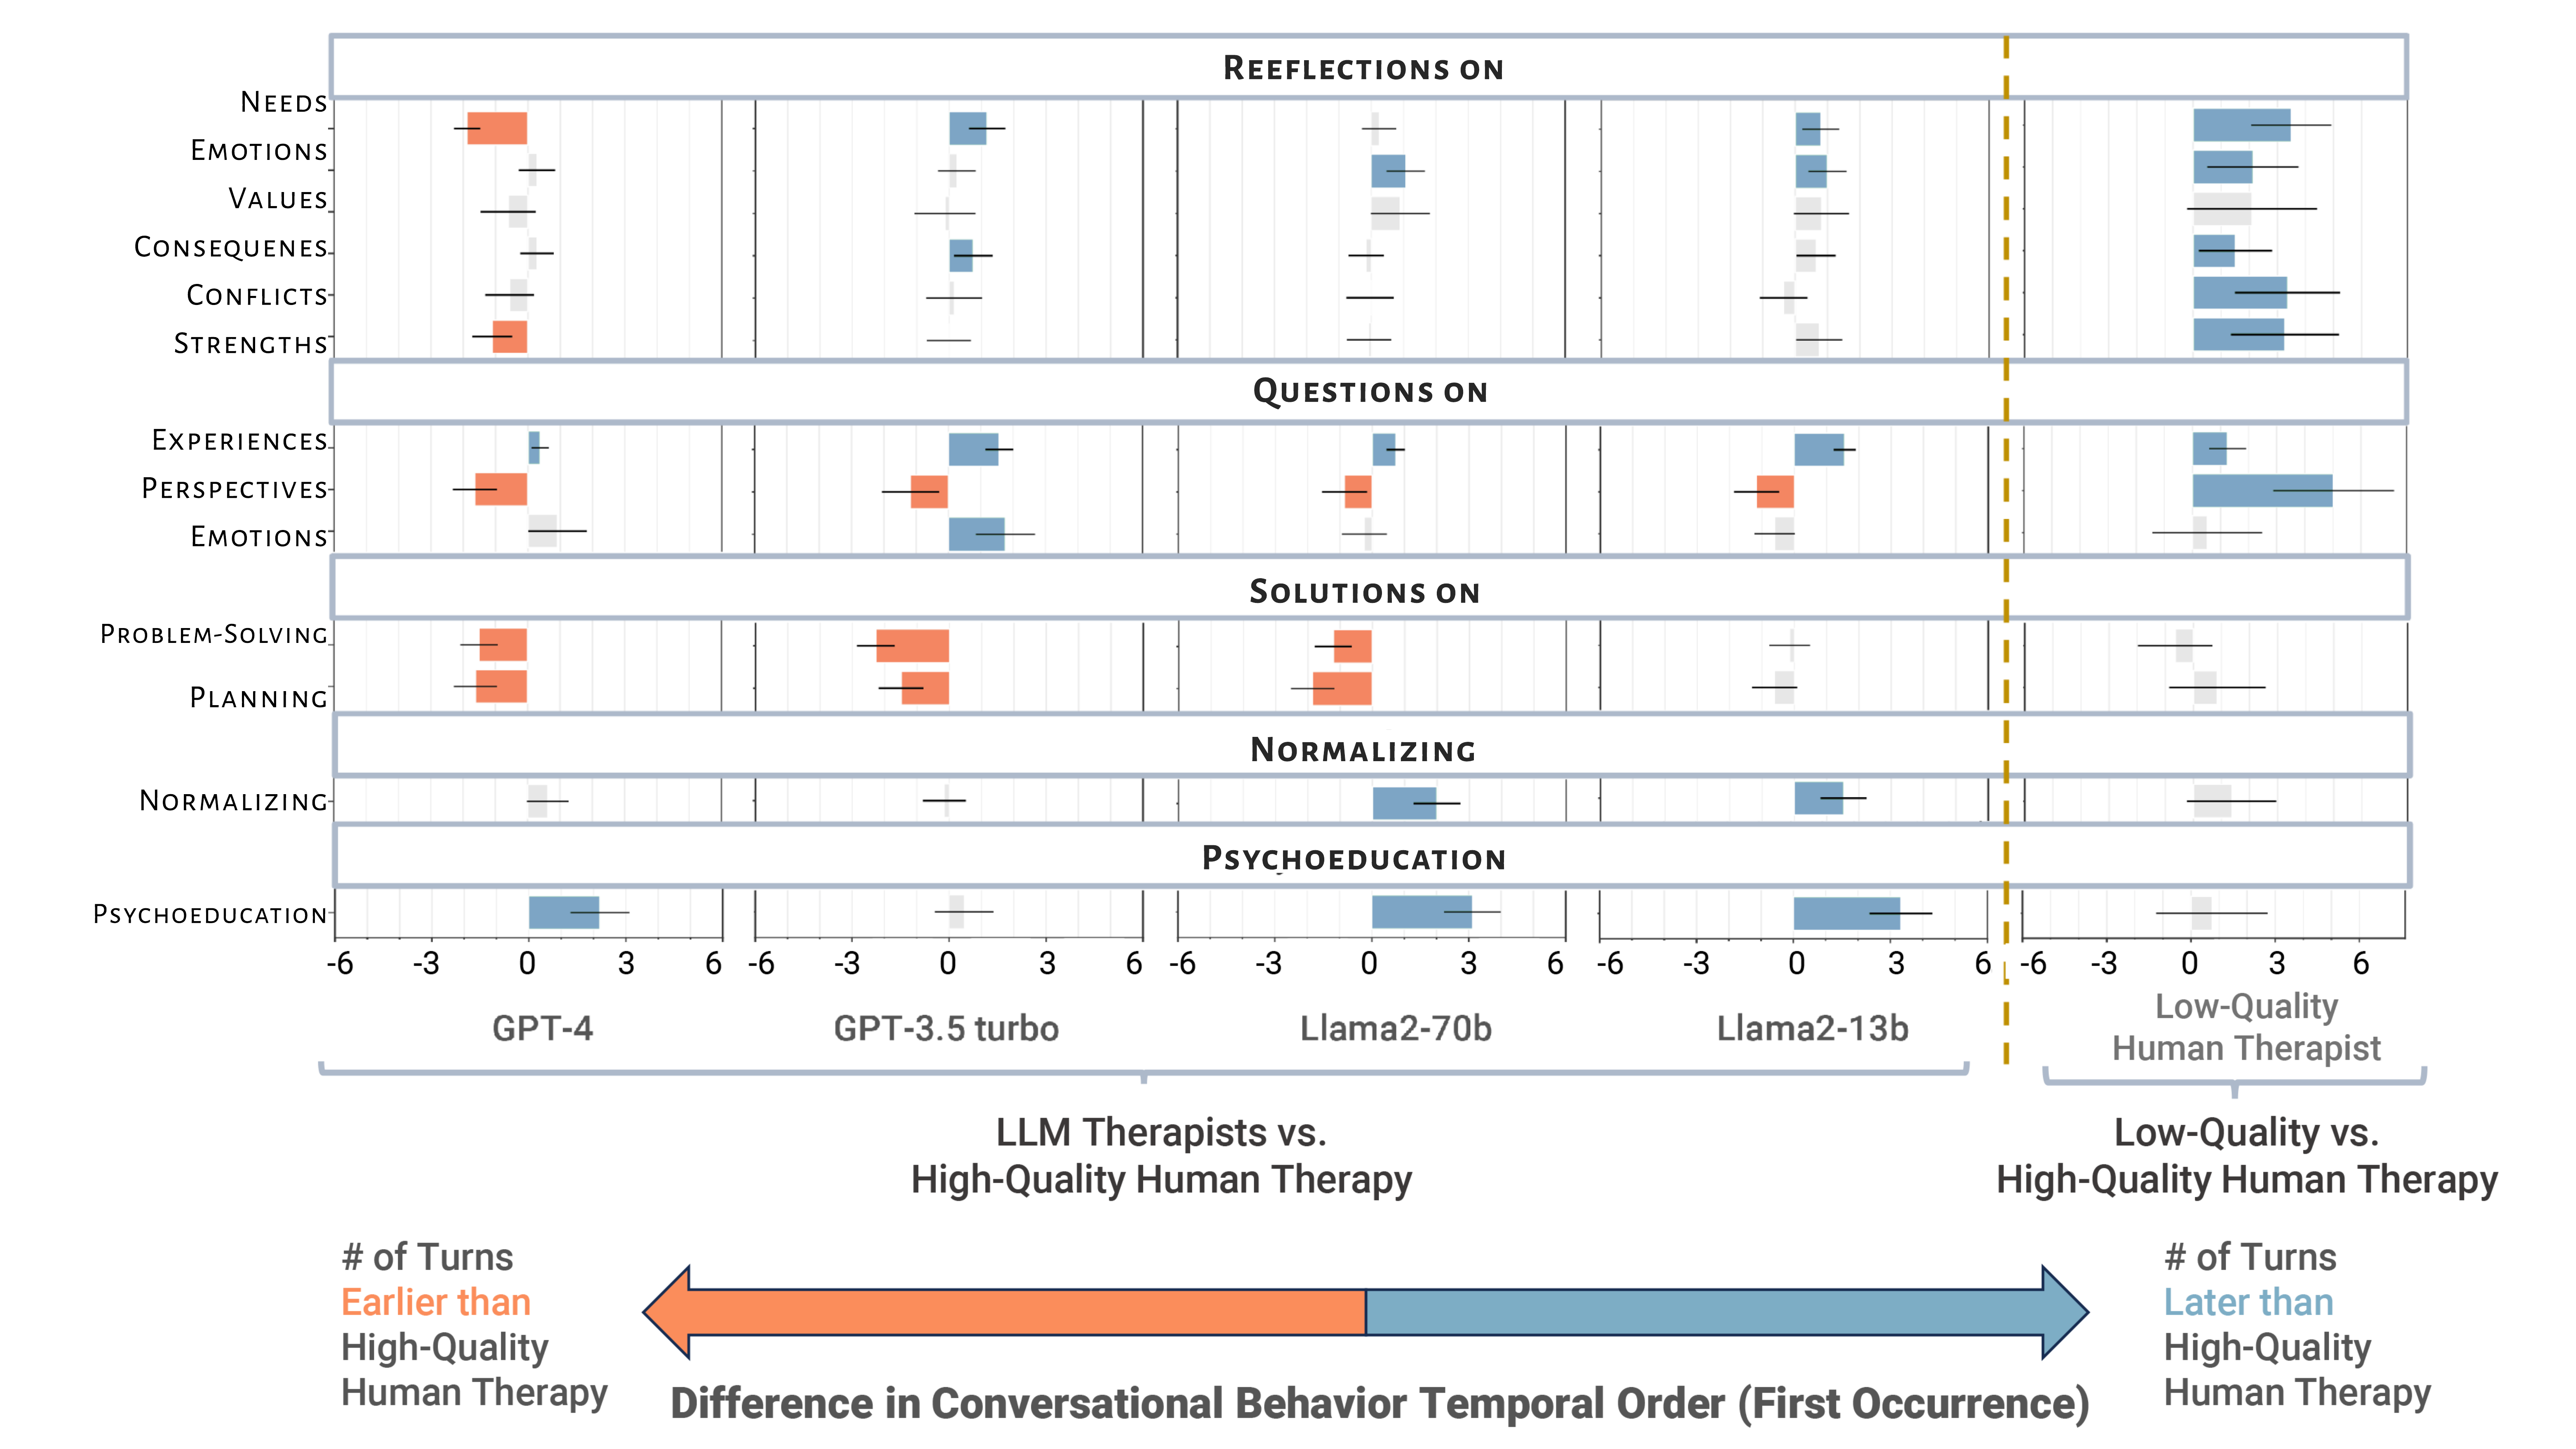}
\centering
\vspace{-10pt}

\caption{Difference in the \textit{temporal order} of conversational behaviors, operationalized as the turn numbers in which behaviors are first exhibited in a conversation by LLM therapists (GPT-4, GPT-3.5-turbo, Llama2-70b, Llama2-13b) or low-quality human therapy, relative to high-quality human therapy. Values $>0$ (highlighted in \textcolor{blueplot}{blue}) indicate that the behavior is first expressed at a later turn whereas Values $<0$ (highlighted in \textcolor{orangeplot}{orange}) indicate that the behavior is first expressed earlier as compared to high-quality human therapy. Values in \textcolor{gray}{gray} are not statistically significantly different from zero at p = 0.05 using Two-sided Student’s t-test. For instance, GPT-4 first responds with \textsc{Problem-Solving} $1.56$ turns earlier than human high-quality therapy. Most LLM therapists start providing \textsc{Solutions} earlier in the conversations, but providing \textsc{Reflections on} client problems later against common recommendations \cite{cochran2015heart}.} 
\vspace{-10pt}
\label{appendix:fig:first_occur_avg}
\end{figure*}
